# Supplementary material for: Poisson Phase Retrieval in Very Low-count Regimes
Source: arXiv:2104.00861 source file (2022-09-24)
Supplement: Supplementary file 1 [file s,appendix.tex]

% s,appendix
% \subsection{Proof of the Improved Curvature}
\label{sec:proof-imp}
